# Supplementary material for: Non equilibrium phase transitions and Floquet Kibble-Zurek scaling
Source: arXiv:1510.08866 ancillary file (2016-11-02)
Supplement: Supplementary file 1 [file Supplemental_Material.pdf]

# Supplemental Material of "Kibble-Zurek Scaling in Periodically-Driven Quantum Systems"

Angelo Russomanno[1,2,3] and Emanuele G. Dalla Torre[1]

[1] *Department of Physics, Bar Ilan University, 52900, Ramat Gan Israel*

[2] *Scuola Normale Superiore, Piazza dei Cavalieri 7, I-56127 Pisa, Italy*

[3] *International Centre for Theoretical Physics (ICTP), Strada Costiera 11, I-34151 Trieste, Italy*

## SM-1. VALIDITY TEST OF THE NUMERICAL METHOD

In this section we analyze the validity of our numerical approach by considering the integrable case $\alpha = 0$, where analytical results are available. In the present calculations the initial state is chosen to be the ground state of the time-averaged Hamiltonian: the static Hamiltonian Eq. (1) of the main text with $h(t) = h_0$. We start our dynamics in the high-frequency limit, where this state is a very good approximation for the Floquet ground state. Due to the presence of a large energy gap (our calculations are performed in the paramagnetic phase of the Ising model), this state is characterized by a low entanglement and is faithfully reproduced by the DMRG code[1]. Fig. S1(a) compares the numerical and analytical results for the time evolution of the entanglement entropy during a slow decrease of the driving frequency $\Omega$. Initially (for $\Omega > 9.3$) the two results overlap, but very soon the numerically-computed entanglement entropy becomes significantly smaller than the exact result.

To understand the causes of this discrepancy we observe that during the present time evolution, the state of the system is characterized by a superposition of the Floquet ground state (FGS), plus a small fraction of Floquet excited states (whose weight goes to zero in the adiabatic limit). In contrast to the FGS, the entanglement of these states tends to infinity in the thermodynamic limit. Although the entanglement entropy is not a linear observable, it is clear that a very small admixture of excited states is sufficient to generate a significant entanglement entropy. The DMRG method is capable of faithfully describing states with low entanglement only and, as a consequence, gives preference to this type of states. The state represented by the DMRG is therefore expected to be closer to the FGS than the one obtained by the exact time evolution. This dramatic effect is shown in Fig. S1(a), where the entanglement entropy predicted by the numerical method (**red** blue points) is seen to approach the entanglement entropy of the Floquet Ground state (**red**green points).

Although the numerically-computed entanglement entropy very soon departs from the exact result, physical quantities are still faithfully described for a much longer time. As explained above, the fast increase of the entanglement entropy of the system is due to the admixture of a small amount of states with a large entropy. The inability of the DMRG method to describe these states does not have a significant impact on physical observables. Fig. S1(b) shows a direct comparison of the transverse magnetization and demonstrates that

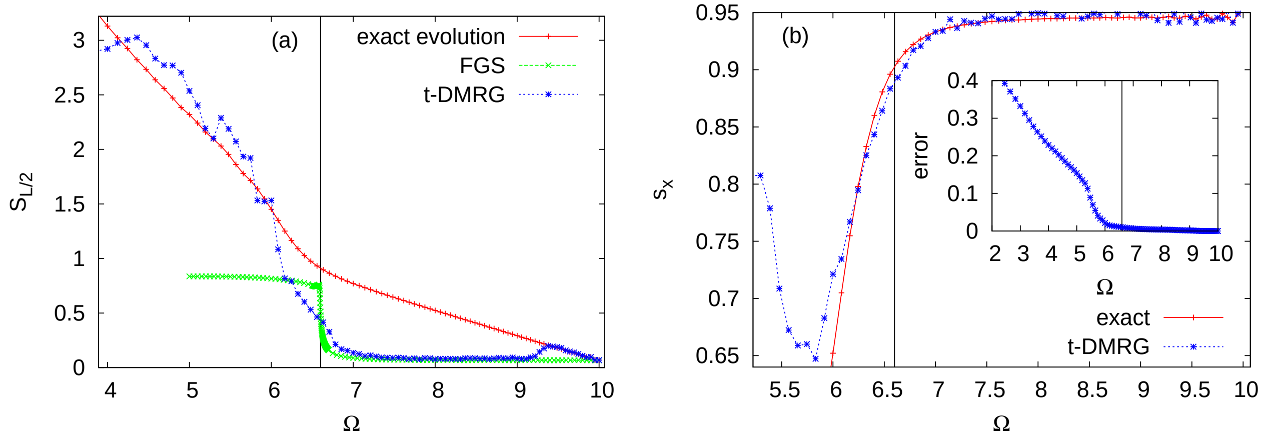


FIG. S1. Comparison between analytical results and numerical evolution for the integrable case ($\alpha = 0$), during a slow decrease of the driving frequency from $\Omega_i = 10$ to $\Omega_f = 4$. (a) Entanglement entropy of half chain: Floquet ground state and evolution with adiabatic change of the frequency (exact results and t-DMRG approximation). (b) Transverse magnetization. (Inset: Cumulative truncation error of the numerical procedure.) In all the plots the vertical line sets the position of the non-equilibrium phase transition occurring at $\Omega = 6.6$. (Numerical parameters: $h_0 = 2.3$, $A = 1.0$, $L = 100$, $t_f = 24\pi$, $\alpha = 0$, open boundary conditions.)

the numerical procedure is valid for all $\Omega > \Omega^* \approx 6$. Note that this frequency is lower than $\Omega_c = 6.6$, allowing us a finite domain of frequencies where the Floquet-Kibble-Zurek scaling can be studied. In the inset of Fig. S1(b) we show the cumulative truncation error of the DMRG method. This quantity is observed to remain very small for all frequencies larger than $\Omega^*$ and to rapidly increase thereafter (for $\Omega < \Omega^*$). In Fig. S2 we repeat the same calculations for a varying system size $L$. For small systems ($L = 25$), the truncation error remains very small (subplot (a)) and the transverse magnetization closely follow the exact, monotonously decreasing, result (subplot (b)). For larger systems, the truncation error is roughly independent on the system size for large frequencies ($\Omega > \Omega^*$), but rapidly increases at smaller frequencies. Starting from this point the value of the transverse magnetization is dominated by the numerical error.

Having performed a direct comparison between the exact and t-DMRG solution of the integrable case, we can infer the validity of the non-integrable case, where only numerical results are available. In Fig. S3 we plot the truncation error and the transverse magnetization along an slow decrease of the frequency, for different values of the system size, in

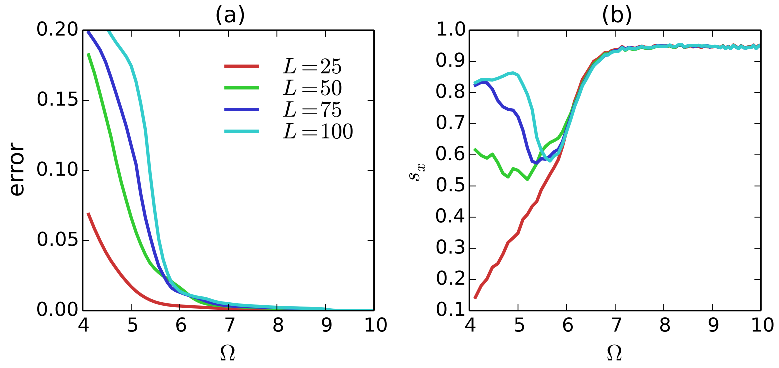


FIG. S2. Finite size effects: and (a) truncation error and (b) transverse magnetization as a function of the instantaneous driving frequency $\Omega$ for different values of the system size, in the integrable case $\alpha = 0$. (Numerical parameters as in Fig. S1)

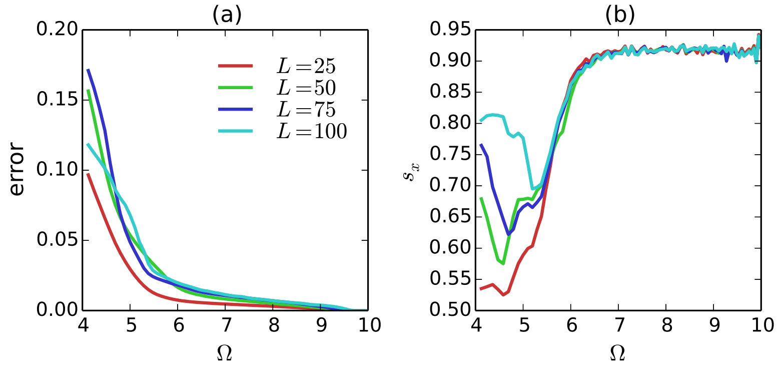


FIG. S3. Same as Fig. S2 for the non-integrable case $\alpha = 0.3$.

the non-integrable case ($\alpha = 0.3$). In analogy to the integrable case, we observe that the truncation error remains small and mainly size-independent for frequencies $\Omega \gtrsim 5.5$. For smaller frequencies the truncation error rapidly grows and local observables depart from the expected value.

In Fig. S4 we study the dependence of the truncation error on the adiabaticity parameter $t_f$. We again observe that the truncation error keeps initially very small and then begins to rapidly increase at $\Omega < \Omega^* \sim 5 - 6$. Interestingly, we observe that in the rescaled plots (subplots (b) and (d)) the position of $\Omega^*$ is found to be roughly constant. For presentation purposes, the region $\Omega < \Omega^*$, where physical observables are not well described by the numerical method, is colored in gray. The same convention is used in Fig. 4 of the main

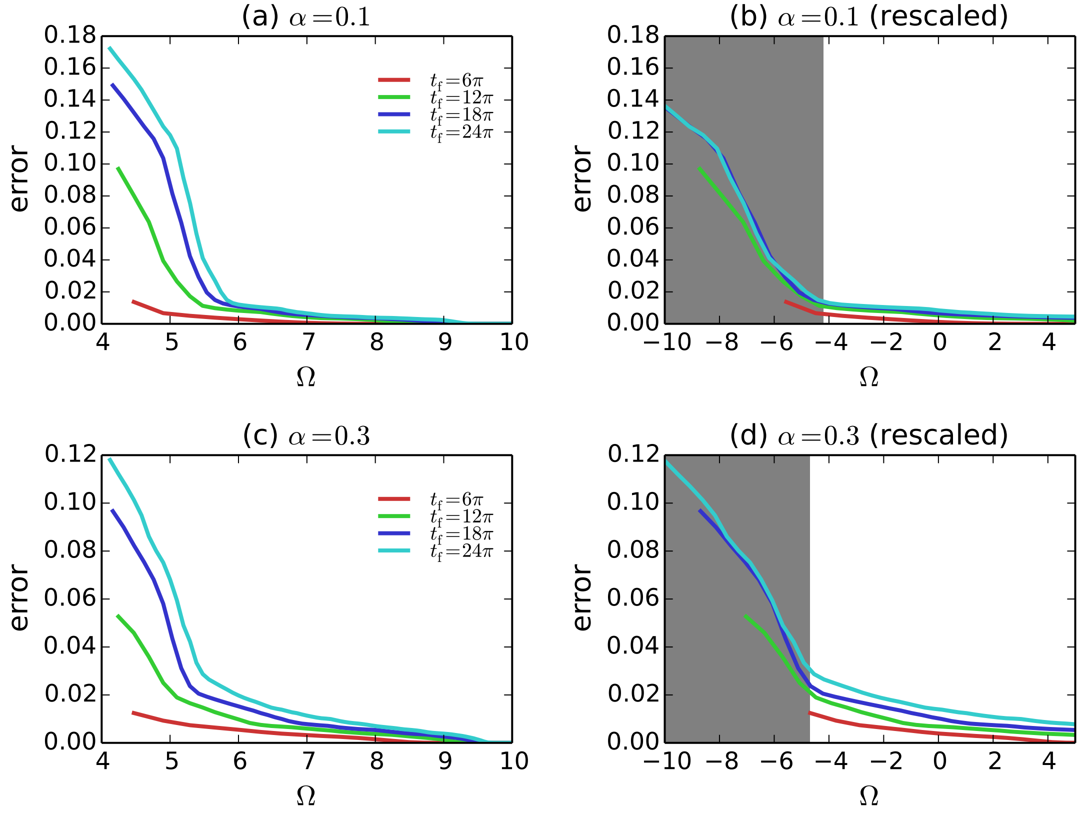


FIG. S4. Cumulative truncation error as a function of the instantaneous driving frequency $\Omega$. The same parameters as in Fig. 4(c-f) of the main text are used.

text, showing the corresponding magnetization.

## SM-2. DETERMINATION OF THE SCALING EXPONENTS

In this section we explain the procedure used to fit the scaling exponents of physical observables. Consider a generic observable $f = f(\Omega, \lambda)$, where $\Omega$ is the driving frequency and $\lambda$ the adiabaticity parameter. According to the Floquet-Kibble-Zurek scaling Ansatz, we expect that for $\lambda \to 0$

$$f(\Omega, \lambda) \approx F\left(\frac{\Omega - \Omega_c}{\lambda^\beta}\right) , \tag{S1}$$

where $\Omega_c$ is the critical frequency at which the Floquet ground state undergoes a quantum phase transition, and $\beta$ is the associated critical exponent. Our goal is now to extract $\beta$ and $\Omega_c$ by comparing the numerical calculations (as a function of $\Omega$) performed for different values of the adiabaticity parameter $\lambda$. In particular, if numerical calculations are performed for

$\lambda_1$ and $\lambda_2$ we will minimize the square Euclidean distance between $F_1(x) = f(\Omega_c + x\lambda_1^\beta, \lambda_1)$ and $F_2(x) = f(\Omega_c + x\lambda_2^\beta, \lambda_2)$, defined as

$$\delta_{12} = \int_{x_a}^{x_b} dx\, (F_1(x) - F_2(x))^2 \ . \tag{S2}$$

The integration boundaries of Eq. (S2) should tend to plus/minus infinity in the limit of $\lambda_{1,2} \to 0$. In the present calculations we achieve this scaling by choosing $x_{a,b} = (\Omega_{a,b} - \Omega_c)/\lambda_2^\beta$ with fixed $\Omega_a$ and $\Omega_b$ (i.e. by fixing the integration boundaries of $f(\Omega, \lambda_2)$). Note that in a periodically driven system $f(\Omega, \lambda)$ is defined only for discrete values of $\Omega$, due to the stroboscopic nature of the problem. To compute the integrated difference Eq. (S2) we first perform a linear interpolation between neighboring frequencies (spline) and then numerically evaluate the integral.

As explained in the text, we here specifically use $f = \mathrm{d}s_x/\mathrm{d}\Omega$ and $\lambda = 1/t_f$, where $s_x$ is the average magnetization per site, and $t_f$ is the time required to reach the final frequency $\Omega_f$. The raw data obtained by the time evolution of the periodic Hamiltonian (1) using the openMPS algorithm (see text for details) is shown in Fig. 4(c) and (e) of the main text. In Fig. S5 we show the distance $\delta_{12}$ (see Eq. (S2)) as a function of the fitting parameters $\Omega_c$ and $\beta$, for two values of the interaction strength $\alpha$ and two distinct pairs of adiabatic parameters $\lambda_1 = 1/t_{f,1}$ and $\lambda_2 = 1/t_{f,2}$. The minimum of this graph is used to determine the optimal values of $\Omega_c$ and $\beta$. We repeated this procedure for all six available pairs of $t_{f,1}$ and $t_{f,2}$ and reported the extracted fitting parameters in Table S1. By averaging over this list we obtain the values of $\Omega_c$ and $\beta$ mentioned in the main text.

## SM-3. NOVELTY OF OUR $t$–DMRG APPROACH

During the last two decades DMRG (and derivatives) have found a large number of applications in computing the equilibrium properties of interacting one-dimensional systems. The validity of this method is justified by the *area-law entanglement* of any state with a finite correlation length, such as the ground state of gapped systems and of disordered (many-body localized) states. In one-dimension, the entanglement of these states does not grow with the system size, allowing computational physicists to analyze very large systems with finite resources.

In contrast, in the case of time-dependent problems, the DMRG method has only found

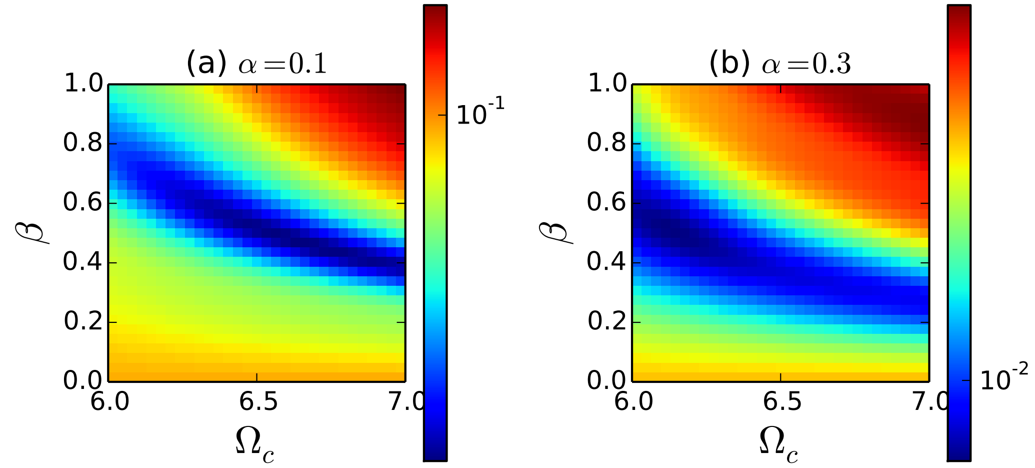


FIG. S5. Square Euclidean distance $\delta_{12}$ (see Eq. (S2)) for (a) $\alpha = 0.1$ and (b) $\alpha = 0.3$. The minimum of these plots is used to extract the fitting parameters $\Omega_c$ and $\beta$ shown in Table S1. Numerical parameters: $\Omega_0 = 10$, $L = 100$, $h_0 = 2.3$, $A = 1.0$, $\Omega_1 = 5.0$, $\Omega_2 = 6.5$, $t_{f,1} = 12\pi$, and $t_{f,1} = 24\pi$.

(a) $\alpha = 0.1$

| $t_{f,1}/\pi$ | $t_{f,2}/\pi$ | $\Omega_c$ | $\beta$ |
|---|---|---|---|
| 6 | 12 | 7.0 | 0.68 |
| 6 | 18 | 6.9 | 0.66 |
| 6 | 24 | 6.5 | 0.36 |
| 12 | 18 | 6.75 | 0.56 |
| 12 | 24 | 6.75 | 0.54 |
| 18 | 24 | 6.7 | 0.38 |
| average | | $6.78 \pm 0.16$ | $0.51 \pm 0.09$ |

(b) $\alpha = 0.3$

| $t_{f,1}/\pi$ | $t_{f,2}/\pi$ | $\Omega_c$ | $\beta$ |
|---|---|---|---|
| 6 | 12 | 7.0 | 0.4 |
| 6 | 18 | 6.8 | 0.4 |
| 6 | 24 | 6.25 | 0.6 |
| 12 | 18 | 7.0 | 0.3 |
| 12 | 24 | 6.3 | 0.5 |
| 18 | 24 | 6.4 | 0.45 |
| average | | $6.6 \pm 0.3$ | $0.44 \pm 0.09$ |

TABLE S1. Optimal fitting parameters for all six available pairs of $t_{f,1}$ and $t_{f,2}$. All other parameters are the same as in Fig. S5.

limited applications, due to the light-cone spreading of correlations and entanglement in the system: when considering a sudden quantum quench, the entanglement entropy generically grows linearly with time and the DMRG method stops to be efficient as soon as time-scales comparable with the inverse interaction strength are reached. In this manuscript, we present a novel example a time-dependent problem where DMRG can be employed to study

the long-time evolution of a many-body systems. Importantly, the present study does not involve the adiabatic change of a quasi-static Hamiltonian (where DMRG supposedly works very well, but little information is added with respect to the study of the associated static problem), but rather a genuine time-dependent problem, in which the parameters of the Hamiltonian change at a frequency comparable to the typical energy scales of the problem. The applicability of the DMRG algorithm to the present study is based on the existence of a low entanglement state in the Floquet spectrum.

From a numerical perspective, the hereby presented protocol is therefore not just one of many possible applications of DMRG methods to study the dynamics of many-body systems, but probably the only one that allows to extend this method to arbitrarily-long time. Furthermore, the existence of a Floquet state with area law entanglement demonstrates the relevance of quantum mechanics to the study of time-dependent many-body systems, and might be employed to generate interesting and useful strongly-correlated states in periodically-driven systems.

## SM-4. EFFECT OF INITIALIZING THE SYSTEM IN THE TIME-AVERAGED GROUND STATE

Throughout the paper we initialize the system in the ground state of the time-averaged Hamiltonian and not in the Floquet ground state. If the initial frequency were infinite, this would not give rise to any problem: the two states wold simply coincide. In contrast, in the present analysis we start from a large *finite* frequency, where the two states are very similar but not equal. This gives rise to some small differences which can be fully appreciated in the integrable case, where it is possible to initialize the system in the Floquet ground state and make a direct comparison with the initialization procedure used in this paper.

To perform this comparison, we plot the excitation density $n_{ex}^{(FGS)}(\Omega)$ when the system is initialized in the initial Floquet ground state. We have to compare this with $n_{ex}(\Omega)$, obtained when the system is initialized in the time-averaged ground state (reported in Fig. 2 of the main text). We see that in the first case $n_{ex}^{(FGS)}(\Omega) = 0$ for $\Omega \gtrsim \Omega_c$ for all $t_f$, leading to a perfect Floquet Kibble-Zurek scaling, while in the second case $n_{ex}^{(FGS)}(\Omega) > 0$ for all $\Omega$ and the scaling is only approximate. In contrast, we observe that the magnetization (Fig. 3(a-b) of the main text) does not change very much if we initialize in the Floquet ground state

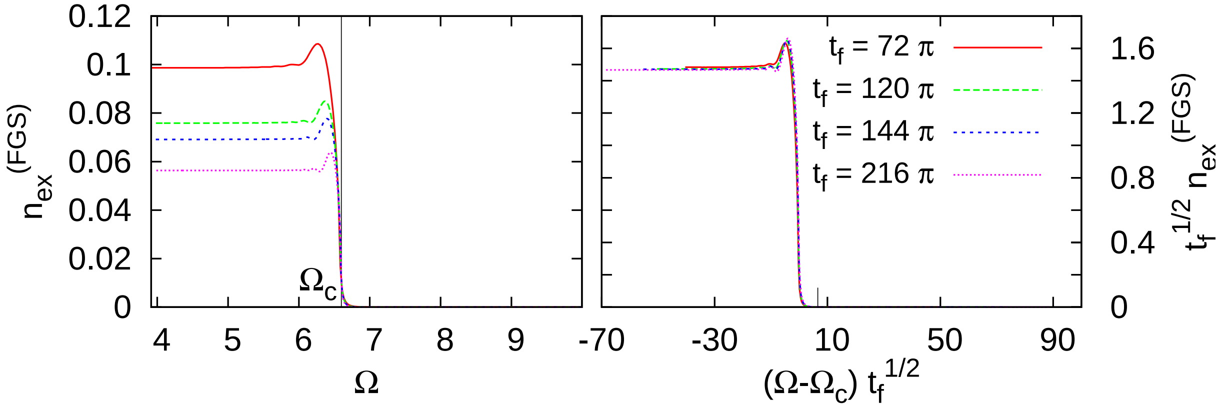


FIG. S6. (Left panel) Number of excitations vs $\Omega$ for different values of $t_f$: it starts increasing after crossing the transition. (Right panel) Kibble-Zurek scaling of the number of excitations: the rescaled curves for different $t_f$ overlap after the rescaling (the overlap is very good because we initialize the system in the Floquet ground state). (Numerical parameters: $h_0 = 2.3$, $A = 1$, $L = 300$, $\Omega_i = 10$, $\Omega_f = 4$; periodic boundary conditions.)

instead of the time-averaged ground state.

---

[1] To make this initialization we use the imaginary-time evolution at a fixed value of $\alpha$.
